# Supplementary material for: Calibrating LLMs for Text-to-SQL Parsing by Leveraging Sub-clause Frequencies
Source: arXiv:2505.23804 source file (2025-09-17)
Supplement: Supplementary file 1 [file possible_additions.tex]

\section{Possible table to add?}

\begin{table*}[ht!]
\centering
\begin{tabular}{c c l c c c c}
\toprule
\textbf{Dataset} & \textbf{Model} & \textbf{Method} 
& \textbf{Brier} ($\downarrow$) & \textbf{ECE} ($\downarrow$) & \textbf{ACE} ($\downarrow$) & \textbf{AUC} ($\uparrow$) \\ 
\toprule

\multirow{6}{*}{SPIDER}

& \multirow{2}{*}{T5 3B}
&   PS          & 0.1626          & 0.0626          & 0.1102          & \textbf{0.8108} \\ 
& & MPS (beam)  & \textbf{0.1545} & \textbf{0.0261} & \textbf{0.0355} & 0.7873          \\

\cmidrule{2-7}

& \multirow{2}{*}{\textsc{Llama 3.1 8B Instruct}}
&   PS          & 0.1736          & 0.0449          & 0.0554          & 0.7260 \\ 
& & MPS (beam)  & \textbf{0.1705} & \textbf{0.0284} & \textbf{0.0344} & \textbf{0.7290} \\

\midrule

\multirow{6}{*}{BIRD}

& \multirow{2}{*}{\textsc{Llama 3.1 8B Instruct}}
&   PS          & 0.2121          & 0.0574          & 0.0737          & 0.6931 \\ 
& & MPS (beam)  & \textbf{0.1990} & \textbf{0.0385} & \textbf{0.0450} & \textbf{0.7195} \\

\cmidrule{2-7}

& \multirow{2}{*}{\textsc{Llama 3.1 70B Instruct}}
&   PS          & 0.2314          & 0.0499          & 0.0652          & 0.6669 \\ 
& & MPS (beam)  & \textbf{0.2211} & \textbf{0.0302} & \textbf{0.0375} & \textbf{0.6932} \\

\bottomrule
\end{tabular}
\caption{
    We report results for model outputs produced using only beam search. To derive sub-clause frequencies from the additional samples in the beam. We observe that \textbf{MPS} out performs \textbf{PS} w.r.t. calibration metrics in all settings. Our results suggest that using beam search, \textbf{MPS} provides improvements for calibration with minimal overhead (i.e., the additional computational workload of prompting the LLM for more samples). We note however that in terms of AUC of error detection, we observe mixed results for the SPIDER dataset, with \textbf{PS} outperforming \textbf{MPS} on outputs produced by \textsc{T5 3B}.
}
\label{tab:calibration+auc_beam}
\end{table*}

\begin{table*}[ht!]
\centering
\begin{tabular}{c c l c c c c}
\toprule
\textbf{Dataset} & \textbf{Model} & \textbf{Method} 
& \textbf{Brier} ($\downarrow$) & \textbf{ECE} ($\downarrow$) & \textbf{ACE} ($\downarrow$) & \textbf{AUC} ($\uparrow$) \\ 
\toprule

\multirow{6}{*}{SPIDER}

& \multirow{2}{*}{\textsc{T5 3B}}
&   PS          & 0.1656 & 0.0622 & 0.0627 & 0.7200 \\ 
& & MPS (nucleus)  & 0.1638 & 0.0460 & 0.0539 & 0.7229          \\

\cmidrule{2-7}

& \multirow{2}{*}{\textsc{Llama 3.1 8B Instruct}}
&   PS          & 0.1740 & 0.0710 & 0.0818 & 0.7241 \\ 
& & MPS (nucleus)  & 0.1637 & 0.0292 & 0.0324 & 0.7449 \\

\midrule

\multirow{6}{*}{BIRD}

& \multirow{2}{*}{\textsc{Llama 3.1 8B Instruct}}
&   PS          & 0.2068 & 0.0501 & 0.1107 & 0.7373 \\ 
& & MPS (nucleus)  & 0.1908 & 0.0354 & 0.0310 & 0.7342 \\

\cmidrule{2-7}

& \multirow{2}{*}{\textsc{Llama 3.1 70B Instruct}}
&   PS          & 0.2274 & 0.0987 & 0.1005 & 0.7244 \\ 
& & MPS (nucleus)  & 0.2069 & 0.0314 & 0.0423 & 0.7416 \\

\bottomrule
\end{tabular}
\caption{
    We report results for model outputs produced using only nucleus sampling. To derive sub-clause frequencies, we use additional outputs produced from bean search only.
}
\label{tab:calibration+auc_nucleus}
\end{table*}

\begin{table*}[ht!]
\centering
\begin{tabular}{lllcccc}
\toprule
\textbf{Method} & \textbf{Score Fn.} & \textbf{Brier} & \textbf{ECE} & \textbf{ACE} & \textbf{AUC} \\
\midrule
\multirow{2}{*}{Uncalibrated}
& Prob. & \textbf{0.1893} & \textbf{0.1632} & \textbf{0.1632} & \textbf{0.7200} \\
& SC & 0.1969 & 0.1706 & 0.1673 & 0.7097 \\
\midrule
\multirow{2}{*}{PS}
& Prob. & \textbf{0.1656} & 0.0623 & 0.0628 & \textbf{0.7200} \\
& SC & 0.1706 & \textbf{0.0620} & \textbf{0.0282} & 0.7097 \\
\midrule
\multirow{2}{*}{MPS (Beam)}
& Prob. & \textbf{0.1565} & \textbf{0.0241} & 0.0308 & \textbf{0.7804} \\
& SC & 0.1594 & 0.0280 & \textbf{0.0293} & 0.7696 \\
\midrule
\multirow{2}{*}{MPS (Nucleus)}
& Prob. & \textbf{0.1639} & \textbf{0.0460} & 0.0538 & \textbf{0.7229} \\
& SC & 0.1673 & 0.0462 & \textbf{0.0176} & 0.7139 \\
\midrule
\multirow{2}{*}{MPS (N + B)}
& Prob. & \textbf{0.1566} & \textbf{0.0264} & \textbf{0.0253} & \textbf{0.7785} \\
& SC & 0.1590 & 0.0273 & 0.0287 & 0.7707 \\
\bottomrule
\end{tabular}
\caption{
    Evaluating on \textsc{T5 3B} on SPIDER, we compare performance of our methods while varying the base scoring function (\textbf{Score Fn.}), choosing between either using model (log sum) token probabilities (\textbf{Prob.}) or using self-consistency (\textbf{SC}), which is derived by checking against the $k=10$ additional outputs produced from nucleus sampling. For methods, we evaluate the uncalibrated scoring functions (\textbf{Uncalibrated}), Platt scaling (\textbf{PS}), and multivariate Platt scaling (\textbf{MPS}) using SCF derived from nucleus sampling only (\textbf{Nucleus}), beam search only (\textbf{Beam}), and both (\textbf{N+B}). We observe little difference between using the two scoring functions.
}
\label{tab:compare_self_consistency_spider_t5}
\end{table*}

%%%%%

\begin{table*}[ht!]
\centering
\begin{tabular}{lllcccc}
\toprule
\textbf{Method} & \textbf{Score Fn.} & \textbf{Brier} & \textbf{ECE} & \textbf{ACE} & \textbf{AUC} \\
\midrule
\multirow{2}{*}{Uncalibrated}
& Prob. & 0.3576 & 0.4161 & 0.4147 & 0.7123 \\
& SC & \textbf{0.3428} & \textbf{0.3732} & \textbf{0.3793} & \textbf{0.7259} \\
\midrule
\multirow{2}{*}{PS}
& Prob. & 0.1726 & 0.0437 & 0.0449 & 0.7123 \\
& SC & \textbf{0.1679} & \textbf{0.0315} & \textbf{0.0315} & \textbf{0.7259} \\
\midrule
\multirow{2}{*}{MPS (Beam)}
& Prob. & 0.1687 & 0.0244 & \textbf{0.0230} & 0.7194 \\
& SC & \textbf{0.1650} & \textbf{0.0222} & 0.0291 & \textbf{0.7400} \\
\midrule
\multirow{2}{*}{MPS (Nucleus)}
& Prob. & 0.1625 & 0.0280 & 0.0360 & 0.7506 \\
& SC & \textbf{0.1612} & \textbf{0.0232} & \textbf{0.0312} & \textbf{0.7557} \\
\midrule
\multirow{2}{*}{MPS (N + B)}
& Prob. & 0.1626 & \textbf{0.0244} & 0.0260 & 0.7475 \\
& SC & \textbf{0.1611} & 0.0257 & \textbf{0.0232} & \textbf{0.7543} \\
\bottomrule
\end{tabular}
\caption{
    Evaluating on \textsc{Llama 3.1 8B Instruct} on SPIDER, we compare performance of our methods while varying the base scoring function (\textbf{Score Fn.}), choosing between either using model (log sum) token probabilities (\textbf{Prob.}) or using self-consistency (\textbf{SC}), which is derived by checking against the $k=10$ additional outputs produced from nucleus sampling. For methods, we evaluate the uncalibrated scoring functions (\textbf{Uncalibrated}), Platt scaling (\textbf{PS}), and multivariate Platt scaling (\textbf{MPS}) using SCF derived from nucleus sampling only (\textbf{Nucleus}), beam search only (\textbf{Beam}), and both (\textbf{N+B}). We observe little difference between using the two scoring functions.
}
\label{tab:compare_self_consistency_spider_llama_8b}
\end{table*}

%%%%%

\begin{table*}[ht!]
\centering
\begin{tabular}{lllcccc}
\toprule
\textbf{Method} & \textbf{Score Fn.} & \textbf{Brier} & \textbf{ECE} & \textbf{ACE} & \textbf{AUC} \\
\midrule
\multirow{2}{*}{Uncalibrated}
& Prob. & \textbf{0.2378} & \textbf{0.1722} & \textbf{0.1688} & \textbf{0.6913} \\
& SC & 0.2574 & 0.2150 & 0.2103 & 0.6577 \\
\midrule
\multirow{2}{*}{PS}
& Prob. & 0.2129 & 0.0556 & 0.0739 & \textbf{0.6913} \\
& SC & \textbf{0.2127} & \textbf{0.0432} & \textbf{0.0586} & 0.6577 \\
\midrule
\multirow{2}{*}{MPS (Beam)}
& Prob. & \textbf{0.1989} & \textbf{0.0425} & \textbf{0.0442} & \textbf{0.7213} \\
& SC & 0.1996 & 0.0428 & 0.0470 & 0.7204 \\
\midrule
\multirow{2}{*}{MPS (Nucleus)}
& Prob. & \textbf{0.1976} & \textbf{0.0574} & \textbf{0.0542} & \textbf{0.7307} \\
& SC & 0.1988 & 0.0588 & 0.0617 & 0.7243 \\
\midrule
\multirow{2}{*}{MPS (N + B)}
& Prob. & \textbf{0.1951} & 0.0418 & 0.0423 & \textbf{0.7347} \\
& SC & 0.1964 & \textbf{0.0408} & \textbf{0.0341} & 0.7301 \\
\bottomrule
\end{tabular}
\caption{
    Evaluating on \textsc{Llama 3.1 8B Instruct} on BIRD, we compare performance of our methods while varying the base scoring function (\textbf{Score Fn.}), choosing between either using model (log sum) token probabilities (\textbf{Prob.}) or using self-consistency (\textbf{SC}), which is derived by checking against the $k=10$ additional outputs produced from nucleus sampling. For methods, we evaluate the uncalibrated scoring functions (\textbf{Uncalibrated}), Platt scaling (\textbf{PS}), and multivariate Platt scaling (\textbf{MPS}) using SCF derived from nucleus sampling only (\textbf{Nucleus}), beam search only (\textbf{Beam}), and both (\textbf{N+B}). We observe little difference between using the two scoring functions.
}
\label{tab:compare_self_consistency_bird_llama_8b}
\end{table*}

%%%%%

\begin{table*}[ht!]
\centering
\begin{tabular}{lllcccc}
\toprule
\textbf{Method} & \textbf{Score Fn.} & \textbf{Brier} & \textbf{ECE} & \textbf{ACE} & \textbf{AUC} \\
\midrule
\multirow{2}{*}{Uncalibrated}
& Prob. & 0.2866 & 0.2343 & 0.2324 & 0.6650 \\
& SC & 0.3264 & 0.3128 & 0.3106 & 0.6798 \\
\midrule
\multirow{2}{*}{PS}
& Prob. & 0.2316 & 0.0549 & 0.0631 & 0.6650 \\
& SC & 0.2273 & 0.0512 & 0.0560 & 0.6798 \\
\midrule
\multirow{2}{*}{MPS (Beam)}
& Prob. & 0.2215 & 0.0384 & 0.0416 & 0.6921 \\
& SC & 0.2182 & 0.0278 & 0.0315 & 0.7047 \\
\midrule
\multirow{2}{*}{MPS (Nucleus)}
& Prob. & 0.2130 & 0.0290 & 0.0267 & 0.7203 \\
& SC & 0.2129 & 0.0304 & 0.0312 & 0.7213 \\
\midrule
\multirow{2}{*}{MPS (N + B)}
& Prob. & 0.1951 & 0.0418 & 0.0423 & 0.7347 \\
& SC & 0.2139 & 0.0224 & 0.0271 & 0.7183 \\
\bottomrule
\end{tabular}
\caption{
    Evaluating on \textsc{Llama 3.1 70B Instruct} on BIRD, we compare performance of our methods while varying the base scoring function (\textbf{Score Fn.}), choosing between either using model (log sum) token probabilities (\textbf{Prob.}) or using self-consistency (\textbf{SC}), which is derived by checking against the $k=10$ additional outputs produced from nucleus sampling. For methods, we evaluate the uncalibrated scoring functions (\textbf{Uncalibrated}), Platt scaling (\textbf{PS}), and multivariate Platt scaling (\textbf{MPS}) using SCF derived from nucleus sampling only (\textbf{Nucleus}), beam search only (\textbf{Beam}), and both (\textbf{N+B}). We observe little difference between using the two scoring functions.
}
\label{tab:compare_self_consistency_bird_llama_70b}
\end{table*}
