# Supplementary material for: Calibrating LLMs for Text-to-SQL Parsing by Leveraging Sub-clause Frequencies
Source: arXiv:2505.23804 source file (2025-09-17)
Supplement: Supplementary file 2 [file calibration+auc_beam.tex]

\begin{table*}[ht!]
\centering
\begin{tabular}{c c l c c c c}
\toprule
\textbf{Dataset} & \textbf{Model} & \textbf{Method} 
& \textbf{Brier} ($\downarrow$) & \textbf{ECE} ($\downarrow$) & \textbf{ACE} ($\downarrow$) & \textbf{AUC} ($\uparrow$) \\ 
\toprule

\multirow{6}{*}{SPIDER}

& \multirow{2}{*}{T5 3B}
&   PS          & 0.1626          & 0.0626          & 0.1102          & \textbf{0.8108} \\ 
& & MPS (beam)  & \textbf{0.1545} & \textbf{0.0261} & \textbf{0.0355} & 0.7873          \\

\cmidrule{2-7}

& \multirow{2}{*}{\textsc{Llama 3.1 8B Instruct}}
&   PS          & 0.1736          & 0.0449          & 0.0554          & 0.7260 \\ 
& & MPS (beam)  & \textbf{0.1705} & \textbf{0.0284} & \textbf{0.0344} & \textbf{0.7290} \\

\midrule

\multirow{6}{*}{BIRD}

& \multirow{2}{*}{\textsc{Llama 3.1 8B Instruct}}
&   PS          & 0.2121          & 0.0574          & 0.0737          & 0.6931 \\ 
& & MPS (beam)  & \textbf{0.1990} & \textbf{0.0385} & \textbf{0.0450} & \textbf{0.7195} \\

\cmidrule{2-7}

& \multirow{2}{*}{\textsc{Llama 3.1 70B Instruct}}
&   PS          & 0.2314          & 0.0499          & 0.0652          & 0.6669 \\ 
& & MPS (beam)  & \textbf{0.2211} & \textbf{0.0302} & \textbf{0.0375} & \textbf{0.6932} \\

\bottomrule
\end{tabular}
\caption{
    We report results for model outputs produced using only beam search. To derive sub-clause frequencies from the additional samples in the beam. We observe that \textbf{MPS} out performs \textbf{PS} w.r.t. calibration metrics in all settings. Our results suggest that using beam search, \textbf{MPS} provides improvements for calibration with minimal overhead (i.e., the additional computational workload of prompting the LLM for more samples). We note however that in terms of AUC of error detection, we observe mixed results for the SPIDER dataset, with \textbf{PS} outperforming \textbf{MPS} on outputs produced by \textsc{T5 3B}.
}
\label{tab:calibration+auc_beam}
\end{table*}
