# Supplementary material for: Calibrating LLMs for Text-to-SQL Parsing by Leveraging Sub-clause Frequencies
Source: arXiv:2505.23804 source file (2025-09-17)
Supplement: Supplementary file 3 [file calibration+auc_nucleus.tex]

\begin{table*}[ht!]
\centering
\begin{tabular}{c c l c c c c}
\toprule
\textbf{Dataset} & \textbf{Model} & \textbf{Method} 
& \textbf{Brier} ($\downarrow$) & \textbf{ECE} ($\downarrow$) & \textbf{ACE} ($\downarrow$) & \textbf{AUC} ($\uparrow$) \\ 
\toprule

\multirow{6}{*}{SPIDER}

& \multirow{2}{*}{\textsc{T5 3B}}
&   PS          & 0.1656 & 0.0622 & 0.0627 & 0.7200 \\ 
& & MPS (nucleus)  & 0.1638 & 0.0460 & 0.0539 & 0.7229          \\

\cmidrule{2-7}

& \multirow{2}{*}{\textsc{Llama 3.1 8B Instruct}}
&   PS          & 0.1740 & 0.0710 & 0.0818 & 0.7241 \\ 
& & MPS (nucleus)  & 0.1637 & 0.0292 & 0.0324 & 0.7449 \\

\midrule

\multirow{6}{*}{BIRD}

& \multirow{2}{*}{\textsc{Llama 3.1 8B Instruct}}
&   PS          & 0.2068 & 0.0501 & 0.1107 & 0.7373 \\ 
& & MPS (nucleus)  & 0.1908 & 0.0354 & 0.0310 & 0.7342 \\

\cmidrule{2-7}

& \multirow{2}{*}{\textsc{Llama 3.1 70B Instruct}}
&   PS          & 0.2274 & 0.0987 & 0.1005 & 0.7244 \\ 
& & MPS (nucleus)  & 0.2069 & 0.0314 & 0.0423 & 0.7416 \\

\bottomrule
\end{tabular}
\caption{
    We report results for model outputs produced using only nucleus sampling. To derive sub-clause frequencies, we use additional outputs produced from bean search only.
}
\label{tab:calibration+auc_nucleus}
\end{table*}
