# Supplementary material for: Calibrating LLMs for Text-to-SQL Parsing by Leveraging Sub-clause Frequencies
Source: arXiv:2505.23804 source file (2025-09-17)
Supplement: Supplementary file 4 [file calibration_results_decode_type.tex]

\begin{table*}[htbp!]
\centering
\begin{tabular}{c c c l c c c}
\toprule
\textbf{Dataset} & \textbf{Model} & \textbf{Decode Type} & \textbf{Method} & \textbf{Brier} & \textbf{ECE} & \textbf{ACE} \\ 
\toprule
\multirow{16}{*}{SPIDER}
& \multirow{8}{*}{T5 3B}
& \multirow{4}{*}{Nucleus}  
&     Token Probs.            & 0.1656           & 0.0622           & 0.0627          \\ 
& & & \quad + Beam            & \textbf{0.1564}  & \textbf{0.0240}  & 0.0307          \\ 
& & & \quad + Nucleus         & 0.1638           & 0.0460           & 0.0539          \\ 
& & & \quad + Nucleus + Beam  & 0.1566           & 0.0265           & \textbf{0.0253} \\
\cmidrule{3-7}
& & \multirow{4}{*}{Beam}
&     Token Probs.            & 0.1626           & 0.0626           & 0.1102          \\ 
& & & \quad + Beam            & \textbf{0.1545}  & 0.0261           & 0.0355          \\ 
& & & \quad + Nucleus         & 0.1615           & 0.0439           & 0.1067          \\ 
& & & \quad + Nucleus + Beam  & 0.1549           & \textbf{0.0256}  & \textbf{0250}   \\ 
\cmidrule{2-7}
& \multirow{8}{*}{\textsc{Llama 3.1 8B Instruct}}
& \multirow{4}{*}{Nucleus}
&     Token Probs.            & 0.1740           & 0.0710           & 0.0818          \\ 
& & & \quad + Beam            & 0.1694           & 0.0341           & 0.0324          \\ 
& & & \quad + Nucleus         & \textbf{0.1637}  & 0.0292           & 0.0324          \\ 
& & & \quad + Nucleus + Beam  & 0.1645           & \textbf{0.0274}  & \textbf{0.0274} \\
\cmidrule{3-7}
& & \multirow{4}{*}{Beam}
&     Token Probs.            & 0.1736           & 0.0449           & 0.0554          \\ 
& & & \quad + Beam            & 0.1705           & 0.0284           & 0.0344          \\ 
& & & \quad + Nucleus         & 0.1638           & \textbf{0.0253}  & \textbf{0.0270} \\ 
& & & \quad + Nucleus + Beam  & \textbf{0.1635}  & 0.0298           & \textbf{0.0270} \\ 
\midrule
\multirow{8}{*}{BIRD}
& \multirow{8}{*}{\textsc{Llama 3.1 8B Instruct}}
& \multirow{4}{*}{Nucleus}
& Token Probs.            & 0.2068           & 0.0501           & 0.1107          \\ 
& &   \quad + Beam            & 0.1920           & 0.0472           & 0.0472          \\ 
& & & \quad + Nucleus         & 0.1908           & \textbf{0.0354}  & \textbf{0.0310} \\ 
& & & \quad + Nucleus + Beam  & \textbf{0.1900}  & 0.0395           & 0.0383          \\
\cmidrule{3-7}
& &   \multirow{4}{*}{Beam}
&     Token Probs.            & 0.2121           & 0.0574           & 0.0737          \\ 
& & & \quad + Beam            & 0.1990           & 0.0385           & 0.0450          \\ 
& & & \quad + Nucleus         & 0.1963           & 0.0552           & 0.0581          \\ 
& & & \quad + Nucleus + Beam  & \textbf{0.1939}  & \textbf{0.0434}  & \textbf{0.0415} \\ 
\bottomrule
\end{tabular}
\caption{
Does decode type affect which method work best? Not really...
}
\label{tab:calibration_decode_type}
\end{table*}

\iffalse

SPIDER - T5
nucleus = 0.7352112676056338
beam = 0.7352112676056338

SPIDER - Llama 8B
nucleus = 0.7476635514018691
beam = 0.7377126654064272

BIRD - Llama 8B
nucleus = 0.3460231135282121
beam = 0.3564625850340136
nucleus + beam = 0.3585415259959487

\fi
