# Supplementary material for: Calibrating LLMs for Text-to-SQL Parsing by Leveraging Sub-clause Frequencies
Source: arXiv:2505.23804 source file (2025-09-17)
Supplement: Supplementary file 5 [file compare_self_consistency.tex]

\begin{table*}[ht!]
\centering
\begin{tabular}{lllcccc}
\toprule
\textbf{Method} & \textbf{Score Fn.} & \textbf{Brier} & \textbf{ECE} & \textbf{ACE} & \textbf{AUC} \\
\midrule
\multirow{2}{*}{Uncalibrated}
& Prob. & \textbf{0.1893} & \textbf{0.1632} & \textbf{0.1632} & \textbf{0.7200} \\
& SC & 0.1969 & 0.1706 & 0.1673 & 0.7097 \\
\midrule
\multirow{2}{*}{PS}
& Prob. & \textbf{0.1656} & 0.0623 & 0.0628 & \textbf{0.7200} \\
& SC & 0.1706 & \textbf{0.0620} & \textbf{0.0282} & 0.7097 \\
\midrule
\multirow{2}{*}{MPS (Beam)}
& Prob. & \textbf{0.1565} & \textbf{0.0241} & 0.0308 & \textbf{0.7804} \\
& SC & 0.1594 & 0.0280 & \textbf{0.0293} & 0.7696 \\
\midrule
\multirow{2}{*}{MPS (Nucleus)}
& Prob. & \textbf{0.1639} & \textbf{0.0460} & 0.0538 & \textbf{0.7229} \\
& SC & 0.1673 & 0.0462 & \textbf{0.0176} & 0.7139 \\
\midrule
\multirow{2}{*}{MPS (N + B)}
& Prob. & \textbf{0.1566} & \textbf{0.0264} & \textbf{0.0253} & \textbf{0.7785} \\
& SC & 0.1590 & 0.0273 & 0.0287 & 0.7707 \\
\bottomrule
\end{tabular}
\caption{
    Evaluating on \textsc{T5 3B} on SPIDER, we compare performance of our methods while varying the base scoring function (\textbf{Score Fn.}), choosing between either using model (log sum) token probabilities (\textbf{Prob.}) or using self-consistency (\textbf{SC}), which is derived by checking against the $k=10$ additional outputs produced from nucleus sampling. For methods, we evaluate the uncalibrated scoring functions (\textbf{Uncalibrated}), Platt scaling (\textbf{PS}), and multivariate Platt scaling (\textbf{MPS}) using SCF derived from nucleus sampling only (\textbf{Nucleus}), beam search only (\textbf{Beam}), and both (\textbf{N+B}). We observe little difference between using the two scoring functions.
}
\label{tab:compare_self_consistency_spider_t5}
\end{table*}

%%%%%

\begin{table*}[ht!]
\centering
\begin{tabular}{lllcccc}
\toprule
\textbf{Method} & \textbf{Score Fn.} & \textbf{Brier} & \textbf{ECE} & \textbf{ACE} & \textbf{AUC} \\
\midrule
\multirow{2}{*}{Uncalibrated}
& Prob. & 0.3576 & 0.4161 & 0.4147 & 0.7123 \\
& SC & \textbf{0.3428} & \textbf{0.3732} & \textbf{0.3793} & \textbf{0.7259} \\
\midrule
\multirow{2}{*}{PS}
& Prob. & 0.1726 & 0.0437 & 0.0449 & 0.7123 \\
& SC & \textbf{0.1679} & \textbf{0.0315} & \textbf{0.0315} & \textbf{0.7259} \\
\midrule
\multirow{2}{*}{MPS (Beam)}
& Prob. & 0.1687 & 0.0244 & \textbf{0.0230} & 0.7194 \\
& SC & \textbf{0.1650} & \textbf{0.0222} & 0.0291 & \textbf{0.7400} \\
\midrule
\multirow{2}{*}{MPS (Nucleus)}
& Prob. & 0.1625 & 0.0280 & 0.0360 & 0.7506 \\
& SC & \textbf{0.1612} & \textbf{0.0232} & \textbf{0.0312} & \textbf{0.7557} \\
\midrule
\multirow{2}{*}{MPS (N + B)}
& Prob. & 0.1626 & \textbf{0.0244} & 0.0260 & 0.7475 \\
& SC & \textbf{0.1611} & 0.0257 & \textbf{0.0232} & \textbf{0.7543} \\
\bottomrule
\end{tabular}
\caption{
    Evaluating on \textsc{Llama 3.1 8B Instruct} on SPIDER, we compare performance of our methods while varying the base scoring function (\textbf{Score Fn.}), choosing between either using model (log sum) token probabilities (\textbf{Prob.}) or using self-consistency (\textbf{SC}), which is derived by checking against the $k=10$ additional outputs produced from nucleus sampling. For methods, we evaluate the uncalibrated scoring functions (\textbf{Uncalibrated}), Platt scaling (\textbf{PS}), and multivariate Platt scaling (\textbf{MPS}) using SCF derived from nucleus sampling only (\textbf{Nucleus}), beam search only (\textbf{Beam}), and both (\textbf{N+B}). We observe little difference between using the two scoring functions.
}
\label{tab:compare_self_consistency_spider_llama_8b}
\end{table*}

%%%%%

\begin{table*}[ht!]
\centering
\begin{tabular}{lllcccc}
\toprule
\textbf{Method} & \textbf{Score Fn.} & \textbf{Brier} & \textbf{ECE} & \textbf{ACE} & \textbf{AUC} \\
\midrule
\multirow{2}{*}{Uncalibrated}
& Prob. & \textbf{0.2378} & \textbf{0.1722} & \textbf{0.1688} & \textbf{0.6913} \\
& SC & 0.2574 & 0.2150 & 0.2103 & 0.6577 \\
\midrule
\multirow{2}{*}{PS}
& Prob. & 0.2129 & 0.0556 & 0.0739 & \textbf{0.6913} \\
& SC & \textbf{0.2127} & \textbf{0.0432} & \textbf{0.0586} & 0.6577 \\
\midrule
\multirow{2}{*}{MPS (Beam)}
& Prob. & \textbf{0.1989} & \textbf{0.0425} & \textbf{0.0442} & \textbf{0.7213} \\
& SC & 0.1996 & 0.0428 & 0.0470 & 0.7204 \\
\midrule
\multirow{2}{*}{MPS (Nucleus)}
& Prob. & \textbf{0.1976} & \textbf{0.0574} & \textbf{0.0542} & \textbf{0.7307} \\
& SC & 0.1988 & 0.0588 & 0.0617 & 0.7243 \\
\midrule
\multirow{2}{*}{MPS (N + B)}
& Prob. & \textbf{0.1951} & 0.0418 & 0.0423 & \textbf{0.7347} \\
& SC & 0.1964 & \textbf{0.0408} & \textbf{0.0341} & 0.7301 \\
\bottomrule
\end{tabular}
\caption{
    Evaluating on \textsc{Llama 3.1 8B Instruct} on BIRD, we compare performance of our methods while varying the base scoring function (\textbf{Score Fn.}), choosing between either using model (log sum) token probabilities (\textbf{Prob.}) or using self-consistency (\textbf{SC}), which is derived by checking against the $k=10$ additional outputs produced from nucleus sampling. For methods, we evaluate the uncalibrated scoring functions (\textbf{Uncalibrated}), Platt scaling (\textbf{PS}), and multivariate Platt scaling (\textbf{MPS}) using SCF derived from nucleus sampling only (\textbf{Nucleus}), beam search only (\textbf{Beam}), and both (\textbf{N+B}). We observe little difference between using the two scoring functions.
}
\label{tab:compare_self_consistency_bird_llama_8b}
\end{table*}

%%%%%

\begin{table*}[ht!]
\centering
\begin{tabular}{lllcccc}
\toprule
\textbf{Method} & \textbf{Score Fn.} & \textbf{Brier} & \textbf{ECE} & \textbf{ACE} & \textbf{AUC} \\
\midrule
\multirow{2}{*}{Uncalibrated}
& Prob. & 0.2866 & 0.2343 & 0.2324 & 0.6650 \\
& SC & 0.3264 & 0.3128 & 0.3106 & 0.6798 \\
\midrule
\multirow{2}{*}{PS}
& Prob. & 0.2316 & 0.0549 & 0.0631 & 0.6650 \\
& SC & 0.2273 & 0.0512 & 0.0560 & 0.6798 \\
\midrule
\multirow{2}{*}{MPS (Beam)}
& Prob. & 0.2215 & 0.0384 & 0.0416 & 0.6921 \\
& SC & 0.2182 & 0.0278 & 0.0315 & 0.7047 \\
\midrule
\multirow{2}{*}{MPS (Nucleus)}
& Prob. & 0.2130 & 0.0290 & 0.0267 & 0.7203 \\
& SC & 0.2129 & 0.0304 & 0.0312 & 0.7213 \\
\midrule
\multirow{2}{*}{MPS (N + B)}
& Prob. & 0.1951 & 0.0418 & 0.0423 & 0.7347 \\
& SC & 0.2139 & 0.0224 & 0.0271 & 0.7183 \\
\bottomrule
\end{tabular}
\caption{
    Evaluating on \textsc{Llama 3.1 70B Instruct} on BIRD, we compare performance of our methods while varying the base scoring function (\textbf{Score Fn.}), choosing between either using model (log sum) token probabilities (\textbf{Prob.}) or using self-consistency (\textbf{SC}), which is derived by checking against the $k=10$ additional outputs produced from nucleus sampling. For methods, we evaluate the uncalibrated scoring functions (\textbf{Uncalibrated}), Platt scaling (\textbf{PS}), and multivariate Platt scaling (\textbf{MPS}) using SCF derived from nucleus sampling only (\textbf{Nucleus}), beam search only (\textbf{Beam}), and both (\textbf{N+B}). We observe little difference between using the two scoring functions.
}
\label{tab:compare_self_consistency_bird_llama_70b}
\end{table*}
